# Supplementary material for: N-ImageNet: Towards Robust, Fine-Grained Object Recognition with Event Cameras
Source: arXiv:2112.01041 source file (2022-03-28)
Supplement: Supplementary file 1 [file supp_all.tex]

\begin{table*}[]
\centering
\resizebox{\textwidth}{!}{
\begin{tabular}{c|c|c|c|c|c|c|c|c}
\hline
Dataset & \begin{tabular}[c]{@{}c@{}}Original\\ Accuracy\end{tabular} & \begin{tabular}[c]{@{}c@{}}Degraded\\ Accuracy\end{tabular} & \multicolumn{6}{c}{Tree Search Accuracy} \\ \hline
\begin{tabular}[c]{@{}c@{}}Search\\ Metric\end{tabular} & - & - & \begin{tabular}[c]{@{}c@{}}Gradient\\ $\uparrow$\end{tabular} & \begin{tabular}[c]{@{}c@{}}Gradient\\ $\downarrow$\end{tabular} & \begin{tabular}[c]{@{}c@{}}Variance\\ $\uparrow$\end{tabular} & \begin{tabular}[c]{@{}c@{}}Variance\\ $\downarrow$\end{tabular} & \begin{tabular}[c]{@{}c@{}}Laplacian\\ $\uparrow$\end{tabular} & \begin{tabular}[c]{@{}c@{}}Laplacian\\ $\downarrow$\end{tabular} \\ \hline
\begin{tabular}[c]{@{}c@{}}Validation\\ Dataset 1\end{tabular} & 48.21\% & 44.44\% & 38.58\% & 46.01\% & 39.87\% & 44.77\% & 38.62\% & 46.09\% \\ \hline
\begin{tabular}[c]{@{}c@{}}Validation\\ Dataset 2\end{tabular} & 48.21\% & 34.60\% & 31.92\% & 38.67\% & 31.79\% & 38.38\% & 31.80\% & 38.77\% \\ \hline
\begin{tabular}[c]{@{}c@{}}Validation\\ Dataset 3\end{tabular} & 48.21\% & 29.59\% & 28.31\% & 26.65\% & 24.90\% & 30.84\% & 26.94\% & 27.94\% \\ \hline
\begin{tabular}[c]{@{}c@{}}Validation\\ Dataset 4\end{tabular} & 48.21\% & 25.44\% & 26.28\% & 24.53\% & 26.69\% & 24.70\% & 26.27\% & 24.67\% \\ \hline
\begin{tabular}[c]{@{}c@{}}Validation\\ Dataset 5\end{tabular} & 48.21\% & 27.65\% & 26.98\% & 28.05\% & 26.94\% & 28.05\% & 26.85\% & 28.18\% \\ \hline
\begin{tabular}[c]{@{}c@{}}Validation\\ Dataset 6\end{tabular} & 48.21\% & 16.25\% & 15.63\% & 12.69\% & 14.47\% & 14.57\% & 14.84\% & 13.49\% \\ \hline
\end{tabular}
}
\caption{Performance degradation and tree search results of 6 channel CNN (all).}
\label{tab:all}
\end{table*}
