# Supplementary material for: N-ImageNet: Towards Robust, Fine-Grained Object Recognition with Event Cameras
Source: arXiv:2112.01041 source file (2022-03-28)
Supplement: Supplementary file 2 [file supp_count.tex]

\begin{table*}[]
\centering
\resizebox{\textwidth}{!}{
\begin{tabular}{c|c|c|c|c|c|c|c|c}
\hline
Dataset & \begin{tabular}[c]{@{}c@{}}Original\\ Accuracy\end{tabular} & \begin{tabular}[c]{@{}c@{}}Degraded\\ Accuracy\end{tabular} & \multicolumn{6}{c}{Tree Search Accuracy} \\ \hline
\begin{tabular}[c]{@{}c@{}}Search\\ Metric\end{tabular} & - & - & \begin{tabular}[c]{@{}c@{}}Gradient\\ $\uparrow$\end{tabular} & \begin{tabular}[c]{@{}c@{}}Gradient\\ $\downarrow$\end{tabular} & \begin{tabular}[c]{@{}c@{}}Variance\\ $\uparrow$\end{tabular} & \begin{tabular}[c]{@{}c@{}}Variance\\ $\downarrow$\end{tabular} & \begin{tabular}[c]{@{}c@{}}Laplacian\\ $\uparrow$\end{tabular} & \begin{tabular}[c]{@{}c@{}}Laplacian\\ $\downarrow$\end{tabular} \\ \hline
\begin{tabular}[c]{@{}c@{}}Validation\\ Dataset 1\end{tabular} & 46.97\% & 43.06\% & 37.02\% & 45.18\% & 38.19\% & 43.67\% & 36.85\% & 45.20\% \\ \hline
\begin{tabular}[c]{@{}c@{}}Validation\\ Dataset 2\end{tabular} & 46.97\% & 34.34\% & 30.70\% & 38.20\% & 30.68\% & 37.74\% & 30.58\% & 38.31\% \\ \hline
\begin{tabular}[c]{@{}c@{}}Validation\\ Dataset 3\end{tabular} & 46.97\% & 28.08\% & 27.32\% & 26.26\% & 24.09\% & 30.34\% & 26.02\% & 27.62\% \\ \hline
\begin{tabular}[c]{@{}c@{}}Validation\\ Dataset 4\end{tabular} & 46.97\% & 24.83\% & 25.39\% & 23.48\% & 25.85\% & 23.79\% & 25.31\% & 23.64\% \\ \hline
\begin{tabular}[c]{@{}c@{}}Validation\\ Dataset 5\end{tabular} & 46.97\% & 26.74\% & 25.72\% & 27.38\% & 25.75\% & 27.28\% & 25.61\% & 27.43\% \\ \hline
\begin{tabular}[c]{@{}c@{}}Validation\\ Dataset 6\end{tabular} & 46.97\% & 15.57\% & 14.86\% & 12.02\% & 13.71\% & 13.78\% & 14.05\% & 12.87\% \\ \hline
\end{tabular}
}
\caption{Performance degradation and tree search results of 4 channel CNN (count).}
\label{tab:count}
\end{table*}
