# Supplementary material for: N-ImageNet: Towards Robust, Fine-Grained Object Recognition with Event Cameras
Source: arXiv:2112.01041 source file (2022-03-28)
Supplement: Supplementary file 3 [file supp_est.tex]

\begin{table*}[]
\centering
\resizebox{\textwidth}{!}{
\begin{tabular}{c|c|c|c|c|c|c|c|c}
\hline
Dataset & \begin{tabular}[c]{@{}c@{}}Original\\ Accuracy\end{tabular} & \begin{tabular}[c]{@{}c@{}}Degraded\\ Accuracy\end{tabular} & \multicolumn{6}{c}{Tree Search Accuracy} \\ \hline
\begin{tabular}[c]{@{}c@{}}Search\\ Metric\end{tabular} & - & - & \begin{tabular}[c]{@{}c@{}}Gradient\\ $\uparrow$\end{tabular} & \begin{tabular}[c]{@{}c@{}}Gradient\\ $\downarrow$\end{tabular} & \begin{tabular}[c]{@{}c@{}}Variance\\ $\uparrow$\end{tabular} & \begin{tabular}[c]{@{}c@{}}Variance\\ $\downarrow$\end{tabular} & \begin{tabular}[c]{@{}c@{}}Laplacian\\ $\uparrow$\end{tabular} & \begin{tabular}[c]{@{}c@{}}Laplacian\\ $\downarrow$\end{tabular} \\ \hline
\begin{tabular}[c]{@{}c@{}}Validation\\ Dataset 1\end{tabular} & 49.41\% & 45.77\% & 42.18\% & 49.08\% & 43.07\% & 47.07\% & 41.64\% & 48.68\% \\ \hline
\begin{tabular}[c]{@{}c@{}}Validation\\ Dataset 2\end{tabular} & 49.41\% & 36.70\% & 34.02\% & 40.99\% & 33.80\% & 40.79\% & 33.71\% & 40.78\% \\ \hline
\begin{tabular}[c]{@{}c@{}}Validation\\ Dataset 3\end{tabular} & 49.41\% & 33.35\% & 31.91\% & 29.45\% & 28.18\% & 33.76\% & 30.15\% & 30.69\% \\ \hline
\begin{tabular}[c]{@{}c@{}}Validation\\ Dataset 4\end{tabular} & 49.41\% & 27.69\% & 27.93\% & 26.20\% & 28.33\% & 25.99\% & 27.54\% & 26.26\% \\ \hline
\begin{tabular}[c]{@{}c@{}}Validation\\ Dataset 5\end{tabular} & 49.41\% & 30.74\% & 30.02\% & 31.46\% & 29.89\% & 31.41\% & 30.04\% & 31.56\% \\ \hline
\begin{tabular}[c]{@{}c@{}}Validation\\ Dataset 6\end{tabular} & 49.41\% & 22.28\% & 17.46\% & 14.10\% & 15.81\% & 16.51\% & 16.59\% & 14.94\% \\ \hline
\end{tabular}
}
\caption{Performance degradation and tree search results of EST.}
\label{tab:est}
\end{table*}
