# Supplementary material for: N-ImageNet: Towards Robust, Fine-Grained Object Recognition with Event Cameras
Source: arXiv:2112.01041 source file (2022-03-28)
Supplement: Supplementary file 4 [file supp_flat.tex]

\begin{table*}[]
\centering
\resizebox{\textwidth}{!}{
\begin{tabular}{c|c|c|c|c|c|c|c|c}
\hline
Dataset & \begin{tabular}[c]{@{}c@{}}Original\\ Accuracy\end{tabular} & \begin{tabular}[c]{@{}c@{}}Degraded\\ Accuracy\end{tabular} & \multicolumn{6}{c}{Tree Search Accuracy} \\ \hline
\begin{tabular}[c]{@{}c@{}}Search\\ Metric\end{tabular} & - & - & \begin{tabular}[c]{@{}c@{}}Gradient\\ $\uparrow$\end{tabular} & \begin{tabular}[c]{@{}c@{}}Gradient\\ $\downarrow$\end{tabular} & \begin{tabular}[c]{@{}c@{}}Variance\\ $\uparrow$\end{tabular} & \begin{tabular}[c]{@{}c@{}}Variance\\ $\downarrow$\end{tabular} & \begin{tabular}[c]{@{}c@{}}Laplacian\\ $\uparrow$\end{tabular} & \begin{tabular}[c]{@{}c@{}}Laplacian\\ $\downarrow$\end{tabular} \\ \hline
\begin{tabular}[c]{@{}c@{}}Validation\\ Dataset 1\end{tabular} & 40.12\% & 38.18\% & 33.63\% & 39.44\% & 33.91\% & 38.95\% & 34.43\% & 38.87\% \\ \hline
\begin{tabular}[c]{@{}c@{}}Validation\\ Dataset 2\end{tabular} & 40.12\% & 33.68\% & 31.29\% & 35.93\% & 31.26\% & 35.70\% & 31.68\% & 35.49\% \\ \hline
\begin{tabular}[c]{@{}c@{}}Validation\\ Dataset 3\end{tabular} & 40.12\% & 26.02\% & 21.74\% & 28.59\% & 19.66\% & 31.32\% & 20.82\% & 29.40\% \\ \hline
\begin{tabular}[c]{@{}c@{}}Validation\\ Dataset 4\end{tabular} & 40.12\% & 26.94\% & 28.84\% & 24.88\% & 29.56\% & 25.09\% & 28.56\% & 24.91\% \\ \hline
\begin{tabular}[c]{@{}c@{}}Validation\\ Dataset 5\end{tabular} & 40.12\% & 29.68\% & 28.56\% & 30.18\% & 29.30\% & 29.86\% & 28.58\% & 30.15\% \\ \hline
\begin{tabular}[c]{@{}c@{}}Validation\\ Dataset 6\end{tabular} & 40.12\% & 22.15\% & 18.65\% & 20.53\% & 17.72\% & 24.84\% & 17.94\% & 22.03\% \\ \hline
\end{tabular}
}
\caption{Performance degradation and tree search results of 1 channel CNN.}
\label{tab:flat}
\end{table*}
