# Supplementary material for: N-ImageNet: Towards Robust, Fine-Grained Object Recognition with Event Cameras
Source: arXiv:2112.01041 source file (2022-03-28)
Supplement: Supplementary file 5 [file supp_time.tex]

\begin{table*}[]
\centering
\resizebox{\textwidth}{!}{
\begin{tabular}{c|c|c|c|c|c|c|c|c}
\hline
Dataset & \begin{tabular}[c]{@{}c@{}}Original\\ Accuracy\end{tabular} & \begin{tabular}[c]{@{}c@{}}Degraded\\ Accuracy\end{tabular} & \multicolumn{6}{c}{Tree Search Accuracy} \\ \hline
\begin{tabular}[c]{@{}c@{}}Search\\ Metric\end{tabular} & - & - & \begin{tabular}[c]{@{}c@{}}Gradient\\ $\uparrow$\end{tabular} & \begin{tabular}[c]{@{}c@{}}Gradient\\ $\downarrow$\end{tabular} & \begin{tabular}[c]{@{}c@{}}Variance\\ $\uparrow$\end{tabular} & \begin{tabular}[c]{@{}c@{}}Variance\\ $\downarrow$\end{tabular} & \begin{tabular}[c]{@{}c@{}}Laplacian\\ $\uparrow$\end{tabular} & \begin{tabular}[c]{@{}c@{}}Laplacian\\ $\downarrow$\end{tabular} \\ \hline
\begin{tabular}[c]{@{}c@{}}Validation\\ Dataset 1\end{tabular} & 46.84\% & 43.58\% & 36.94\% & 45.31\% & 38.00\% & 44.12\% & 36.95\% & 45.42\% \\ \hline
\begin{tabular}[c]{@{}c@{}}Validation\\ Dataset 2\end{tabular} & 46.84\% & 34.45\% & 31.22\% & 38.46\% & 31.03\% & 38.21\% & 31.03\% & 38.45\% \\ \hline
\begin{tabular}[c]{@{}c@{}}Validation\\ Dataset 3\end{tabular} & 46.84\% & 28.81\% & 28.07\% & 26.91\% & 24.81\% & 31.08\% & 26.86\% & 28.29\% \\ \hline
\begin{tabular}[c]{@{}c@{}}Validation\\ Dataset 4\end{tabular} & 46.84\% & 25.44\% & 26.17\% & 24.64\% & 26.60\% & 24.87\% & 26.19\% & 24.78\% \\ \hline
\begin{tabular}[c]{@{}c@{}}Validation\\ Dataset 5\end{tabular} & 46.84\% & 27.97\% & 26.92\% & 28.72\% & 26.80\% & 28.78\% & 26.94\% & 28.84\% \\ \hline
\begin{tabular}[c]{@{}c@{}}Validation\\ Dataset 6\end{tabular} & 46.84\% & 17.21\% & 16.40\% & 13.75\% & 14.94\% & 16.29\% & 15.53\% & 14.59\% \\ \hline
\end{tabular}
}
\caption{Performance degradation and tree search results of 4 channel CNN (time).}
\label{tab:time}
\end{table*}
